# Supplementary material for: AEGNN: Asynchronous Event-based Graph Neural Networks
Source: arXiv:2203.17149 source file (2022-11-01)
Supplement: Supplementary file 1 [file appendix.tex]

\documentclass[10pt,twocolumn,letterpaper]{article}

\usepackage{cvpr}              %

\usepackage{graphicx}
\usepackage{amsmath}
\usepackage{amssymb}
\usepackage{booktabs}
\usepackage{lipsum}
\usepackage{float}  %
\usepackage{subfig}  %
\usepackage[accsupp]{axessibility}

\usepackage{pifont}

\usepackage{xcolor}

\usepackage[pagebackref,breaklinks,colorlinks]{hyperref}

\usepackage{color}

\usepackage[capitalize]{cleveref}
\crefname{section}{Sec.}{Secs.}
\Crefname{section}{Section}{Sections}
\Crefname{table}{Table}{Tables}
\crefname{table}{Tab.}{Tabs.}

\makeatletter
\makeatother

\title{Supplementary Material --- AEGNN: Asynchronous\\ Event-based Graph Neural Networks}

\begin{document}

\author{Simon Schaefer\thanks{these authors contributed equally}
\quad\quad\quad
Daniel Gehrig$^*$
\quad\quad\quad
Davide Scaramuzza \\ \\
Dept. Informatics, Univ. of Zurich and \\
Dept. of Neuroinformatics, Univ. of Zurich and ETH Zurich
}
\maketitle

\input{latex/appendix_text.tex}

{\small
\bibliographystyle{ieee_fullname}
\bibliography{all}
}

\end{document}
